# Supplementary material for: On Reinforcement Learning and Distribution Matching for Fine-Tuning Language Models with no Catastrophic Forgetting
Source: arXiv:2206.00761 source file (2022-11-14)
Supplement: Supplementary file 1 [file codegeneration.tex]

\section{Code generation with compilability constraints experiments}

\subsection{Experimental setup}

\paragraph{Energy-based model}
We represent a language model producing only compilable sequences as the following  product-of-experts \citep{Hinton02} EBM:
\begin{equation}
    P(x) = a(x)b(x),
\end{equation}
where $a$ is the original language model pre-trained using a standard autoregressive language modeling objective and $b(x) = 1$ iff $x$ is a syntactically correct Python program and $b(x) = 0$ otherwise.

\paragraph{Dataset}
In contrast with experiments with GPT-2, we trained a custom language model to obtain $a$. To prepare the training dataset for $a$,  we started from the Python150 dataset, which consists of 150k Python source code files obtained from GitHub \cite{Raychev2016}. We extracted 713k Python functions (both methods and standalone functions) from 150k using the code from \citet{roziere2020unsupervised} while filtering out functions that didn't compile ($b(x) = 0$) or were less than 128 BPE tokens long. We then split the dataset into a training subset $\mathcal{D}_\text{train}$ and test subset $\mathcal{D}_\text{test}$.

\paragraph{Initial language model $a$:}
We implemented $a$ using the GPT-2 \cite{radford2019language} architecture with 117m parameters (\texttt{gpt2-small}). First, we used $\mathcal{D}_\text{train}$ to train a byte-level BPE tokenizer. We included two special tokens, BOS and EOS, and obtained a vocabulary of 50k tokens. Then, we trained $a$ on $\mathcal{D}_\text{train}$ for one epoch.

\paragraph{Compilability Scorer $b$}
We evaluate whether a sample $x$ is compilable by first removing BOS and EOS tokens and then calling the \texttt{compile\_command} function from \texttt{codeop} module of Python Standard Library\footnote{\url{https://docs.python.org/3/library/codeop.html}} with $x$ as the argument.  \texttt{compile\_command} tries to compile a string of Python code and raises and exception if there is it fails (e.g. raises \texttt{SyntaxError} for invalid Python syntax and \texttt{ValueError} or \texttt{OverflowError} if there is an invalid literal in $x$). If \texttt{compile\_command} returns a \texttt{code} object, $b(x)=1$. Otherwise (if an exception is raised or \texttt{None} is returned), $b(x)=0$. Note that our notion of compilability is concerned only with syntactic correctness and does not execute the body of a function.

\subsection{Metrics}

In addition to $\E_{x \sim \pit} b(x)$, $\KL(p, \pit)$, $\KL(\pit, a)$, Distinct-1  \citep{li-etal-2016-diversity} and Self-BLEU-5 \citep{texygen-ZhuLZGZWY18}, we report the following metrics:
\begin{enumerate}
    \item Perplexity measured on $\mathcal{D}_\text{test}$, a held-out subset of the data used for training $a$, calculated as 
    $$
    \exp \Big [ - \frac{1}{N}  \sum_{x \in \mathcal{D}_\text{test}} \log \pit(x) \Big],
    $$
    where $N$ is the total number of tokens in $\mathcal{D}_\text{test}$.
    \item Sequence length, the average number of characters in generated sequence $x$ after detokenization,
    \item AST node count, the average number of nodes in an abstract syntax tree (AST) of sequences that compile. Samples are parsed to their corresponding ASTs using the \texttt{ast} module from Python Standard Library.\footnote{\url{https://docs.python.org/3/library/ast.html}} Intuitively, this metric indicates the logical (as opposed to surface) complexity of generated programs.
\end{enumerate}

\subsection{Results}

We report the performance of GDC and GDC++ as well as Reinforce on Table \ref{appendix:code-gen-table}.

Reinforce with $R(x) = b(x)$ improves compilability but that comes at a cost of large divergence from $p$ and $a$. This divergence translates into a decrease in sequence length and logical complexity (in terms of the number of nodes in ASTs of generated sequences). Heavily decreased sequence length (most of the generated functions are one-liners) accounts for an artificial increase in diversity metrics (Self-BLEU-5 and Distinct-1).

GDC and GDC++ are the only method that consistently improve compilability rate while decreasing divergence from $p$, maintaining the diversity of $a$ and only slightly decreasing sequence length and the number of nodes in ASTs. Moreover, as a by-product of improving compilability, GDC and GDC++ are also able to slightly decrease the perplexity and the frequency of PEP8 violations per character. The addition of baseline in GDC++ improves its performance in terms of constraint satisfaction, KL divergences and downstream metrics (e.g. lower Self-BLEU-5, higher Distinct-1).

% comment how reinforce (Reward Maximization) converges to very short sentences wrt AST node cound and Length. 

\begin{table}[H]
\footnotesize
\begin{tabular}{lrrrrrrrrr}
\toprule
{} &  Ctrl. ($\uparrow$) &  $\text{KL}(p,\pi)$ ($\downarrow$) &  $\text{KL}(\pi,a)$ ($\downarrow$) &  Dist-1 ($\uparrow$) & SB-5 ($\downarrow$) &  AST &  Length &  PPL ($\downarrow$) \\
\midrule
\gc{Original LM}         & \gc{0.55} &  \gc{0.58} & \gc{0.00} & \gc{0.37} &  \gc{0.88} &    \gc{31.40} &   \gc{156.70} & \gc{8.72} \\
Reinforce  &       \textbf{0.89} & 77.49 & 93.26 & 0.52 &  0.79 &    13.21 &   60.23 & 9.32 \\
GDC        &       0.68 &  0.48 &  0.15 & 0.36 &  0.89 &    26.16 &   125.83 & 8.69 \\
GDC++      &       \underline{0.69} &  \underline{\textbf{0.46}} &  \underline{\textbf{0.13}} & 0.36 &  \underline{0.88} &   25.93 &   124.20 & 8.70 \\
% code-generation-reinforceP &       1.00 & 12.57 & 16.65 & 0.15 &  1.00 &    14.00 &   2.00 &     75.00 &       10.75 \\
\bottomrule
\end{tabular}
\caption{\small{  Evaluation of GDC \citep{khalifa_2021}, GDC++ (ours) and Reinforce for python code generation under compilability constraints.
      The best method (excluding ties) overall is highlighted in \textbf{bold}, while the best method between GDC and GDC++ is \underline{underlined}.
   }}
  \label{appendix:code-gen-table}
\end{table}
