# Supplementary material for: On Reinforcement Learning and Distribution Matching for Fine-Tuning Language Models with no Catastrophic Forgetting
Source: arXiv:2206.00761 source file (2022-11-14)
Supplement: Supplementary file 3 [file GDC_intro_experiments.tex]

We investigate the benefits of the proposed DPG variant on the Generation with Distributional Control (GDC)~\citep{khalifa_2021} technique, which makes use of DPG to control the properties of pre-trained language models.

Here, we follow the formulation of~ \citet{A-parshakova-etal-2019-global} and \citet{khalifa_2021}, in which 
the EBM $P(x)$ is implicitly defined by the condition that its normalized counterpart $p(x)=P(x)/Z$, where $Z=\sum_x P(x)$, minimizes the KL divergence $\KL(p,a)$ from an original pretrained language model $a$, while matching a set of desired moments constraints on certain given features $\phi_i(x)$.
These constraints are expressed as conditions $\bar{\mu}_i = \EX{x \sim p} \phi_i(x)$, for $i \in \{1,\dots,n\}$, by which the moments (expectations) under the distribution $p$ of each feature $\phi_i(x)$ are required to take certain desired values $\bar{\mu}_i$.
%Generally,  given set of $n$ moment constraints:
%$$\EX{x \sim p} \phi_1(x) = \bar{\mu}_1, \ldots,\: \EX{x \sim p} \phi_n(x) = \bar{\mu}_n,
%$p$ can be shown to be uniquely determined as the normalized distribution $p(x) = \frac{1}{Z} P(x)$, with $Z = \sum_x P(x)$, where $P(x)$ is an EBM~\citep{lecun_tutorial_2006} of the (exponential family) form:%

Then, $P(x)$ can be shown to be uniquely determined by an EBM~\citep{lecun_tutorial_2006} of the following (exponential family) form\footnote{For a more precise formulation of this EBM, see \citep{khalifa_2021}.}:
\begin{equation} 
    P(x) = a(x)e^{\sum_{i=1}^n \lambda_i \phi_i(x)}. \label{eq:target-EBM}
\end{equation}

The $\lambda_i$ terms control the moments $\mu_i$ of the associated features, which can be estimated through self-normalized importance sampling \citep{owen_chapter_importance_sampling_2013}; and then, to make the moments match the desired values, the $\lambda_i$ terms can be optimized through SGD~\citep{A-parshakova-etal-2019-global}.
%for controlled NLG / Khalifa

For controlled language generation, \citet{khalifa_2021} define $\phi_i$ as binary classifiers of certain properties of a sequence $x$ such as the topic, gender or sentiment. For instance, let $\phi_1(x) = 1$ iff the topic of $x$ is science and $\phi_2(x) = 1$ iff $x$ mentions a female person, then imposing moments $\bar{\mu}_1 = 1$ and $\bar{\mu}_2 = 0.5$ constrains the language model $p$ to only generate sequences about science, half of which mention females.
% for data efficient learning /  Parshakova
In the case of \citet{A-parshakova-etal-2019-global} these moment constraints $\bar{\mu}_i$ are defined to match certain feature expectations of the training data, and the prior knowledge resulting from ``paying attention'' to these features leads to a more data-efficient learning.

%Here the $\lambda_i$'s are parameters ensuring moment matching, which can be estimated from a large sample from $a$ through self-normalized importance sampling \citep{A-parshakova-etal-2019-global,KimBengio2016,owen_chapter_importance_sampling_2013}.
%
% The equation for snis is incomplete (sum over i). I think we can avoid entering into this aspect here.
% by minimizing the mean-square error between desired moments $\bar{\mu}_i$ and estimated moments $\hat{\mu}_i = \frac{\sum_n^N \exp{(\lambda_i \phi_i(x))} \phi_i(x)}{\sum_n^N \exp{(\lambda_i \phi_i(x))}}$, based on $N$ samples obtained through self-normalized importance sampling \citep{KimBengio2016,A-parshakova-etal-2019-global}.
%
%
%
%
