# Supplementary material for: On Reinforcement Learning and Distribution Matching for Fine-Tuning Language Models with no Catastrophic Forgetting
Source: arXiv:2206.00761 source file (2022-11-14)
Supplement: Supplementary file 4 [file KL-DPG-EBM-comparison.tex]

% \section{Comparison Between EBMs forms in GDC and KL-Control}
% \label{appenix:ziegler-dpg}


% \paragraph{Comparison of GDC (with one distributional constraint) and Ziegler}
% %% MD: I find this paragraph to be misleading. Will explain orally.
% % In the general case, $p_Z$ is different from $p$. However, in a special case of a single constraint and when setting $\beta = \frac{1}{\lambda}$, they are equivalent:
% % \begin{equation}
% %     p(x) = \frac{1}{Z}a(x)e^{\lambda \phi(x)} = \frac{1}{Z} a(x)e^{r(x)/\beta} = p_Z(x)
% % \end{equation}
% % Unfortunately, in practice, nothing in Ziegler's objective or adaptive schedule for $\beta$ encourages $\beta$ to approximate $\frac{1}{\lambda}$.

% % This connection could be made more general if we redefine Ziegler's reward $r(x)$ as $r'(x) = \sum_i \lambda_i \phi_i$ for a proper choice of $\lambda_i$s. 

% % The direction of the KL divergence turns out to be crucial. 

% Let's now consider a special case of GDC, with a single binary feature $\phi(x)$ and with a distributional moment constraint $\E_{x\sim p} \phi(x) = \bar{\mu}$, where $\bar{\mu} < 1.0$. Then we know \citep{khalifa_2021} that the optimal distribution for GDC has the form:
% \begin{align*}
%     p(x) \propto a(x) e^{\lambda.\phi(x)},
% \end{align*}
% where $\lambda$ has been determined based on $\bar{\mu}$, the moment constraint that we want to impose. 

% If now we define a ``reward'' $r(x) \doteq \phi(x)$, and \emph{fix} the hyperparameter $\beta$ to the value $1/\lambda$, then the optimal solution for Ziegler, $p_Z$, coincides with the optimal solution $p$ for GDC. In other words, providing a moment specification in GDC forces a choice for Ziegler's free hyperparameter $\beta$. It is interesting to note that, while the departure points of GDC and Ziegler are different --- with, arguably, an advantage to GDC, which provides a directly interpretable specification: matching the expectations of features to  empirical or externally imposed expectations --- they lead to a similar form of EBM.%
% %\md{Hesitation: should we mention the fact --- that we could exploit in another publication --- that this connection opens the way for using \eqref{eq:Rtz} as the basis for a competitor algorithm to DPG? Note that the fact this is possible is related to a special behavior of the $\Rtz$ as defined here. (And reciprocally, we could use DPG for Ziegler!!!)}


% \paragraph{The case of a pointwise constraint}
% Pointwise constraints in GDC do not lead to an exponential form of the optimal EBM and the comparison with Ziegler needs to be treated apart.

% We illustrate in Figure \ref{fig:Geometry-Ziegler-Reinforce} the case a single pointwise binary constraint $\phi$ and desired moment $\bar{\mu} = 1$. Let the manifold $\mathcal{C}$ be the set of distributions $c$ that put probability mass only on sequences satisfying the constraint, i.e. $c(x) > 0 \Rightarrow \phi(x)=1$, or, equivalently such that $\E_{x\sim c} \phi(x) = 1$. DPG's optimal $p$, which for a single pointwise binary constraint takes the form $a(x)\phi(x)$,\footnote{See \citep[Theorem 1B]{khalifa_2021}} lies on $\mathcal{C}$ by definition, while having minimal KL divergence from~$a$.

%  Reinforce, however, will have its reward maximized on \emph{any} distribution $p_R$ on $\mathcal{C}$. On the other hand, for Ziegler, each temperature $\beta$ is associated with an optimal distribution $p_Z = \frac{1}{Z} a(x)e^{r(x)/\beta}$.
% $p_Z$ cannot lie on $\mathcal{C}$, because it gives positive probability to all sequences $x$ in the support of $a$, including points $x$ not satisfying $\phi(x) = 1$. 

% % It wouldn't for $\beta \to 0_+$, when it would be equivalent to $p$.

% \begin{figure}[H]
% \centering
% \includegraphics[trim=0 35 0 125,width=0.7\linewidth]{figures//p_and_reinforce_and-ziegler_2.pdf}
% \caption{A geometric illustration of the relation between $a$ and the policies and Reinforce ($p_R$), Ziegler ($p_Z$) and DPG ($p$). The curved lines represent increasing levels of the KL divergence $\KL(\cdot,a)$ and $\mathcal{C}$ is the manifold associated with $\phi$. Figure adapted from \citep{khalifa_2021}.}
% \label{fig:Geometry-Ziegler-Reinforce}
% \end{figure}
