# Supplementary material for: On Reinforcement Learning and Distribution Matching for Fine-Tuning Language Models with no Catastrophic Forgetting
Source: arXiv:2206.00761 source file (2022-11-14)
Supplement: Supplementary file 10 [file table_comparison.tex]

\begin{table*}[h]
    \centering
\begin{tabular}{l c c }
\toprule
 & \textbf{DPG} & \textbf{\DPGoff} \\
\midrule
 \textbf{Reward} & 
 $\frac{P(x)}{\pi_\theta(x)}$ & 
 $\frac{P(x)}{q(x)}$\\
 \addlinespace
 \textbf{$\nabt$} & 
{\small $\E_{x \sim \pit} \frac{P(x)}{\pi_\theta(x)} \nabt \log \pit(x)$} & 
{\small $\E_{x \sim q} \frac{P(x)}{q(x)} \nabt  \log \pit(x)$} \\ 
 \addlinespace
 \textbf{Baseline}& 
 $Z$   & 
 $Z\frac{\pit(x)}{q(x)}$\\
 \addlinespace
 \addlinespace
 \textbf{Advantage} & 
 $\frac{P(x)}{\pi_\theta(x)} - Z$ & 
 $\frac{P(x)}{q(x)} - Z\frac{\pit(x)}{q(x)}$ \\
 \addlinespace
 \textbf{$\nabt$ with baseline} & 
 {\small $\E_{x \sim \pit} \Big[ \frac{P(x)}{\pi_\theta(x)} - Z \Big] \nabt \log \pit(x)$} & 
{\small $\E_{x \sim q} \Big[ \frac{P(x)}{q(x)} - Z\frac{\pit(x)}{q(x)} \Big] \nabt  \log \pit(x)$} \\
 \bottomrule
\end{tabular}
    \caption{\small{A comparison of Online DPG and Offline DPG (\DPGoff)} forms of Reward, Baseline, Advantage, and Gradient of the loss function (the PG-term) before ($\nabla_\theta$) and after ($\nabla_\theta$ with Baseline) including a baseline for variance reduction.}
    \label{tab:my_label}
\end{table*}
